# Supplementary material for: Cytoskeletal Anisotropy Controls Geometry and Forces of Adherent Cells
Source: arXiv:1702.03916 ancillary file (2018-11-01)
Supplement: Supplementary file 1 [file SI_Pomp_Schakenraad_2018.pdf]

# Cytoskeletal anisotropy controls geometry and forces of adherent cells Supplementary information


Wim Pomp,[1] Koen Schakenraad,[2,3] Hayri E. Balcıoğlu,[4] Hedde van Hoorn,[1] Erik H. J. Danen,[4] Roeland M. H. Merks,[3,5] Thomas Schmidt,[1] and Luca Giomi[2]

[1] *Kamerlingh Onnes-Huygens Laboratory, Leiden University, Niels Bohrweg 2, 2333 CA, Leiden, The Netherlands*
[2] *Instituut-Lorentz, Leiden University, P.O. Box 9506, 2300 RA Leiden, The Netherlands*
[3] *Mathematical Institute, Leiden University, P.O. Box 9512, 2300 RA Leiden, The Netherlands*
[4] *Toxicology, Leiden Academic Center for Drug Research, Leiden University, The Netherlands*
[5] *Institute of Biology, Leiden University, P.O. Box 9505 2300 RA Leiden, The Netherlands*


## SUPPLEMENTARY DATA

### Curvature variation

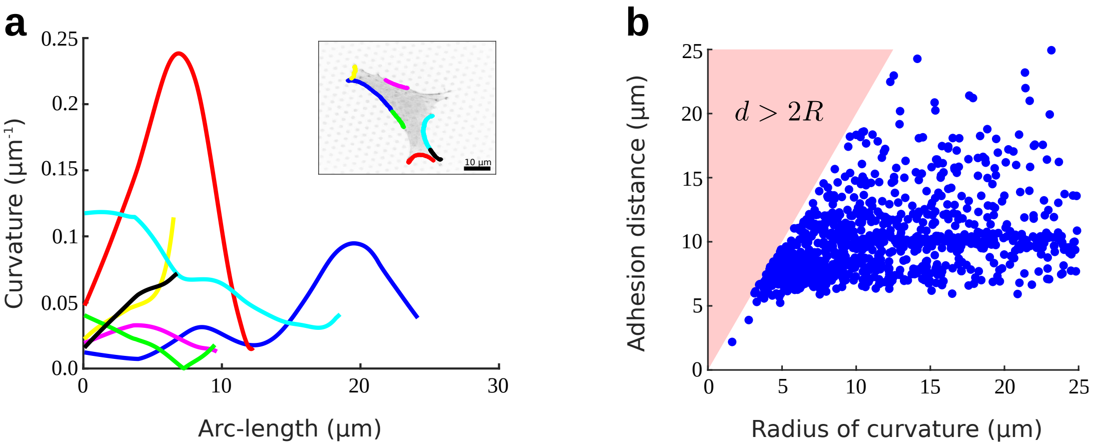


FIG. S1. (a) Curvature versus arc-length for a specific cell (inset).sThe blue, red, cyan, yellow and black arcs are evidently non-circular as indicated by the smooth curvature variation. Because any smooth plane curve can be locally approximated by a circle of radius $R = 1/\kappa$, longer arcs are more likely to exhibit appreciable curvature variations. The large curvature variation of the yellow arc is instead caused by the fact that the arc is roughly perpendicular to the stress fibers, hence it experiences the largest anisotropy in the force distribution. (b) Average radius of curvature of a cellular arc versus the distance between the end-points of the arc (i.e. adhesion points). The radius of curvature is obtained by fitting cellular arcs with circles (see Fig. 1 in the main text and Fig. S2). The data points correspond to a sample of 285 cells and do not allow conclusive statements about a possible correlation between the arcs length and curvature.

### Material parameters for different cell types

The letter which this supplementary accompanies gives the material parameters $\gamma$, $\lambda_{\rm min}$, $\sigma$ and $\alpha$ for a set of 285 cells. These cells, in fact, come from a pool of two different cell types [14,15]. The GE11 cells used exhibit an epithelioid morphology whereas the GD25 cells exhihbit a fibroblastoid morphology. Both cell types are deficient of the fibronectin receptor integrin β1. In both cell types then either α5β1 was reexpressed, or αvβ3 was expressed. These cells are designated GEβ1, GEβ3, GDβ1 and GDβ3. The differing cell and integrin types result in a different cell-substrate coupling leading to different material parameters for each cell and integrin expression type. It is outside the scope of this Letter to examine these differences in detail, therefore initially only the average of each parameter over all 285 cells is given. For completeness, we give the same parameters per cell type in Supplementary Table S1. As can be expected [14], cells expressing β1 exert higher traction forces than cell expressing β3, which is reflected in a lower $\lambda_{\rm min}$ for the latter.

| Cell type | number of cells | $\gamma$ | $\lambda_{\min}$ (nN) | $\sigma$ (nN/μm) | $\alpha$ (nN/μm) |
|---|---|---|---|---|---|
| GEβ1 | 59 | $0.32 \pm 0.14$ | $9.8 \pm 6.9$ | $1.4 \pm 1.0$ | $2.6 \pm 2.2$ |
| GEβ3 | 112 | $0.31 \pm 0.19$ | $5.5 \pm 3.4$ | $0.62 \pm 0.41$ | $1.3 \pm 1.1$ |
| GDβ1 | 56 | $0.38 \pm 0.26$ | $10.6 \pm 9.4$ | $0.92 \pm 0.78$ | $1.5 \pm 1.7$ |
| GDβ3 | 58 | $0.34 \pm 0.25$ | $7.9 \pm 6.0$ | $1.0 \pm 0.8$ | $2.0 \pm 2.2$ |
| All | 285 | $0.33 \pm 0.20$ | $7.6 \pm 5.6$ | $0.87 \pm 0.70$ | $1.7 \pm 1.7$ |

TABLE S1. Survey of the average material parameters per cell type in a sample of 285 fibroblastoid and epithelioid cells. Shown are the mean and standard deviation. Whereas $\gamma$ does not vary significantly, there is some variance observed in especially $\lambda_{\min}$, which appears larger for cells expressing β-integrin.

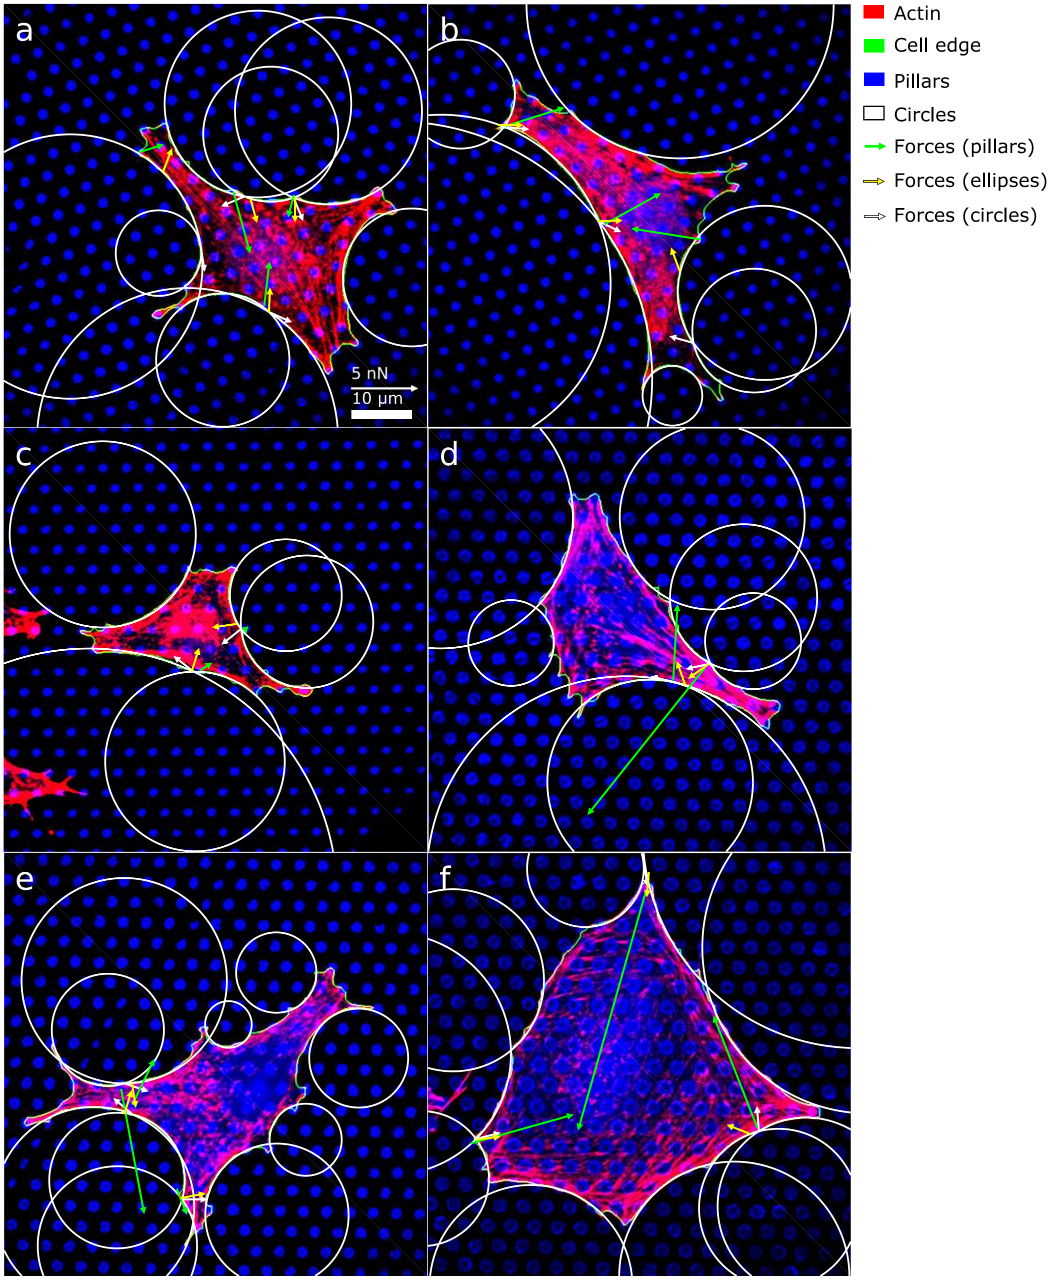


FIG. S2. Six examples of cells with circles fitted to the cell edges. The actin, cell edge and micropillar tops are in the red, green and blue channels respectively. Circles (white) are fitted to the edge of the cells. The arrows correspond to the measured forces (green) and predicted directions (but not magnitudes) of the forces in the presence of isotropic ($\alpha = 0$, white arrow) and anisotropic ($\alpha \neq 0$, yellow arrow) contractile stresses. Green arrows originate from the center of the micropillar, while yellow and white arrows originate from the intersections of ellipses and circles respectively, therefore, arrows do not necessarily originate from the same point. Yellow and white arrows are only plotted for adhesion points under an intersection of ellipses or circles respectively. Panels (a) to (c) show epithelioid cells and (d) to (f) show fibroblastoid cells.

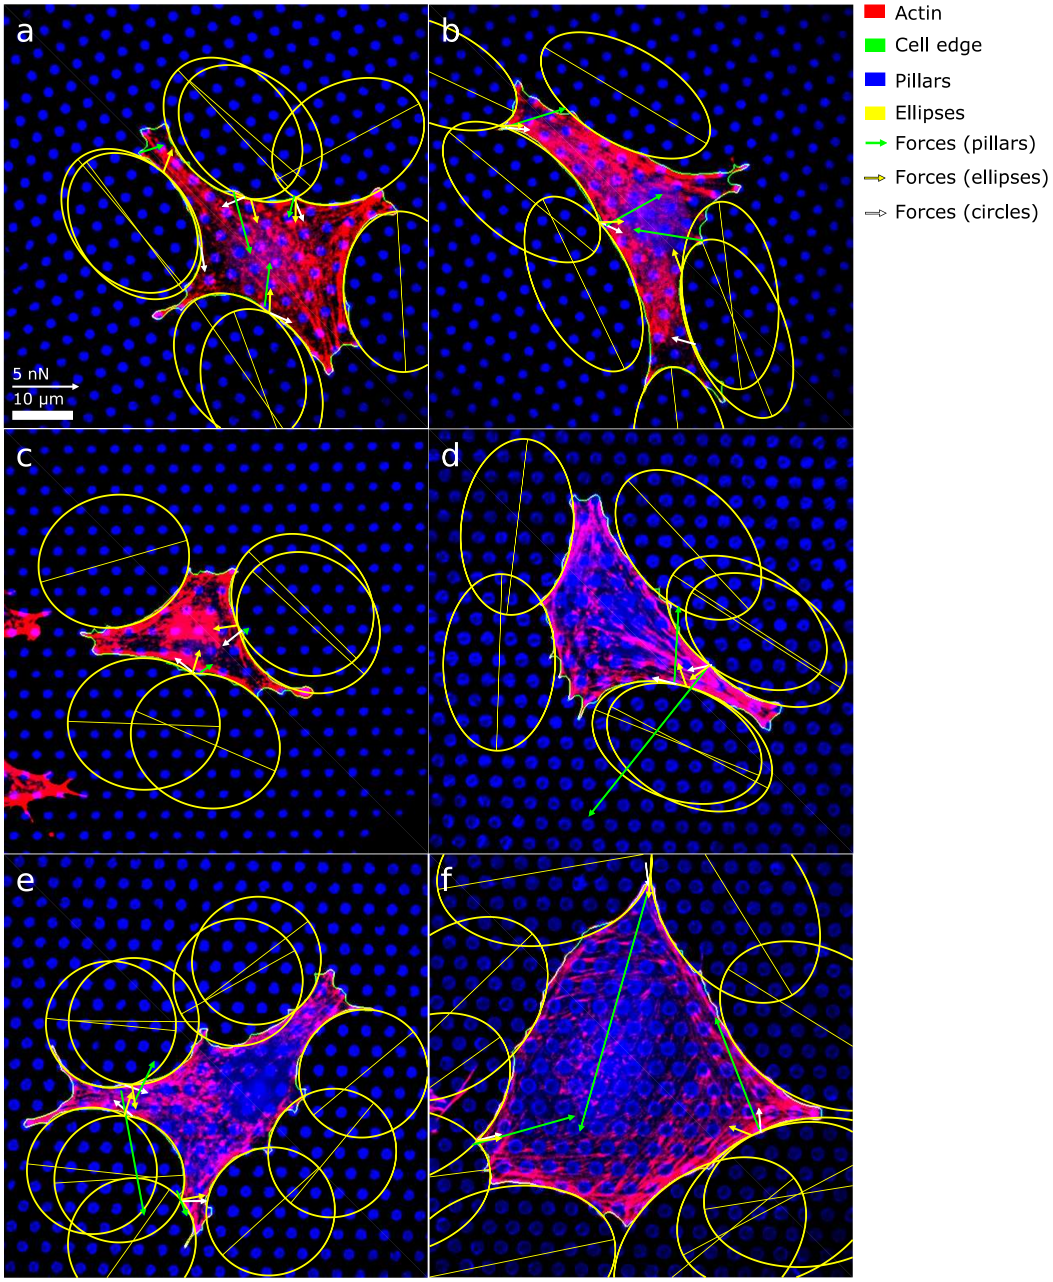


FIG. S3. Six examples of cells (same as in figure S2) with ellipses fitted to the cell edges. The actin, cell edge and micropillar tops are in the red, green and blue channels respectively. Ellipses (yellow, including the major axis) are fitted to the edge of the cells. The arrows correspond to the measured forces (green) and predicted directions (but not magnitudes) of the forces in the presence of isotropic ($\alpha = 0$, white arrow) and anisotropic ($\alpha \neq 0$, yellow arrow) contractile stresses. The length of the green arrows indicates the magnitude of the force. Green arrows originate from the center of the micropillar, while yellow and white arrows originate from the intersections of ellipses and circles respectively, therefore, arrows do not necessarily originate from the same point. Yellow and white arrows are only plotted for adhesion points under an intersection of ellipses or circles respectively. Panels (a) to (c) show epithelioid cells and (d) to (f) show fibroblastoid cells. Fit values for the ellipses in panels (a) to (f) respectively: $\gamma$: 0.52; 0.25; 0.75; 0.40; 0.95; 0.46, $\lambda_{\min}/\sigma$ (μm): 13.4; 15.7; 12.6; 14.7; 10.8; 18.0.

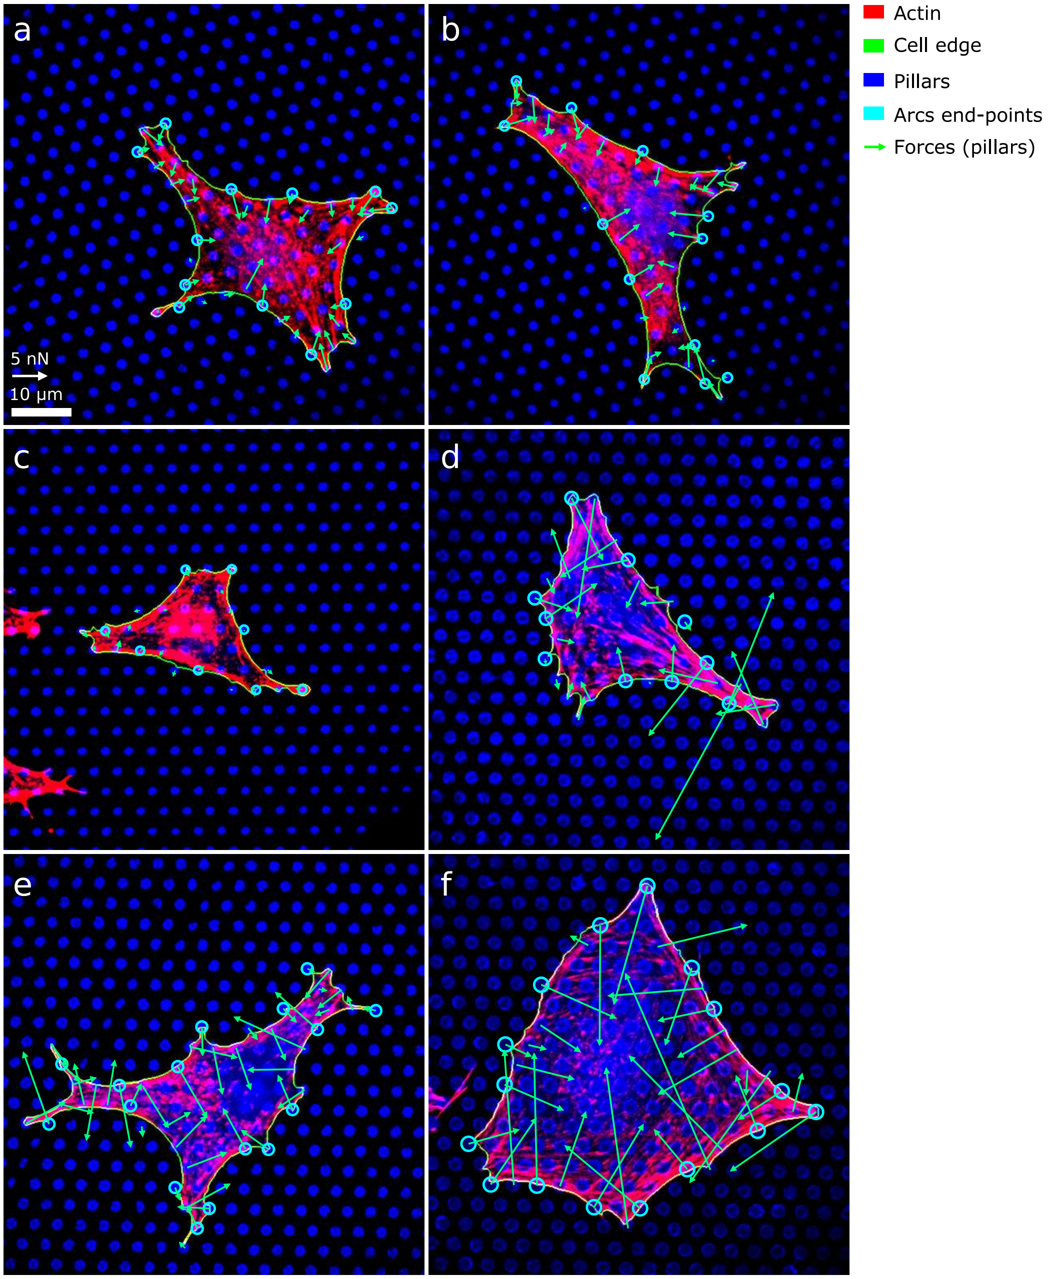


FIG. S4. Six examples of cells (same as in Figs. S2 and S3) with all the traction forces measured along the contour explicitly indicated. The actin, cell edge and micropillar tops are in the red, green and blue channels respectively. The length of the green arrows indicates the magnitude of the force and the pillars used for the geometrical fits, illustrated in Figs. S2 and S3 are highlighted. Panels (a) to (c) show epithelioid cells and (d) to (f) show fibroblastoid cells.

## METHODS

### Cell culture and fluorescent labelling

Epithelioid GE11 and fibroblastoid GD25 cells [26] expressing either α5β1 or αvβ3 (GDβ1, GDβ3, GEβ1 and GEβ3) have been cultured as described before [18]. GDβ1, GDβ3, GEβ1 and GEβ3 are approximately equally represented among the 285 cells in the data presented here. Cells have cultured in medium (DMEM; Dulbecco's Modified Eagle's Medium, Invitrogen/Fisher Scientific) supplemented with 10% fetal bovine serum (HyClone, Etten-Leur, The Netherlands), 25 U/ml penicillin and 25 μg/ml streptomycin (Invitrogen/Fisher Scientific cat. # 15070-063). Cells were fixed in 4% formaldehyde and then permeabilised with 0.1% Triton-X and 0.5% BSA in PBS. Tetramethylrhodamine (TRITC)-Phalloidin (Fisher Emergo B.V. cat. # A12380, Thermo Fisher) was subsequently used to stain F-actin.

### Micropillar arrays

Micropillar arrays were made out of a soft elastomeric material (PDMS) using a negative silicon wafer as a mask as described before [28,29]. Briefly, the 2 μm diameter micropillars are arranged in a hexagonal pattern with a 4 μm centre-to-centre distance. The micropillars have a height of 6.9 μm, resulting in a stiffness of 16.2 nN/μm. The pillar tops were fluorescently labelled using an Alexa 405-fibronectin conjugate (Alexa Fluor®, Invitrogen/Fisher Scientific, Breda, The Netherlands; Fibronectin cat. #1141, Sigma Aldrich, Zwijndrecht, The Netherlands). Pillar deflections were determined with ∼30 nm precision using a specifically designed Matlab script resulting in a ∼0.5 nN precision in force [29].

### Imaging

High-resolution imaging was performed on an in-house constructed spinning disk confocal microscope based on an Axiovert200 microscope body with a Zeiss Plan-Apochromat 100× 1.4NA objective (Zeiss, Sliedrecht, The Netherlands) and a CSU-X1 spinning disk unit (CSU-X1, Yokogawa, Amersfoort, The Netherlands). Imaging was done using an emCCD camera (iXon 897, Andor, Belfast, UK). Alexa405 and TRITC were exited using 405 nm (Crystalaser, Reno, NV) and 561 nm (Cobolt, Stockholm, Sweden) lasers, respectively. This results in a resolution of approximately 150 nm and 200 nm respectively, enough to distinguish separate stress fibers which are typically separated by about 1.5 μm.

### Image analysis

All image analysis and ellipse fitting are performed using Matlab®, except the determination of the stress fibre orientation, for which ImageJ with the OrientationJ plugin (`http://bigwww.epfl.ch/demo/orientation`) was used. The micropillar array allows measuring forces that the cell exerts on the substrate. The pillars used for the force calculations and the geometrical fit shown in Figs. S2 and S3 we selected according to the following criteria. *1)* They are within 10 pixels (1.38 μm) from the edge of the cell. *2)* They are subject to a force that is at least 3 times larger than the average force on all the pillars or such that the tangent vector along the cell contour rotates by an angle equal or larger than 30°. *3)* The distance between two pillars delimiting the same ellipse is larger than 50 pixels (6.9 μm). Fig. S4 show examples of the pillars identified with these criteria for the six cells displayed in Figs. S2 and S3.

### Ellipse fitting

Ellipses are defined in our experiments with five parameters each: the coordinates of the centre of the ellipse, the minor and major semi-axes, and the angle that the major axis of the ellipse makes with the $x-$axis of the coordinate system of the image. We use fixed lengths for major and minor axes for the $N$ ellipses in the same cell. The optimal ellipse size per cell and positions for each ellipse are found using a $2(N+1)$ parameter fit which minimises the distance between fitted ellipses and cell edge by calculating $\chi^2$. Initial parameters for this fit are obtained from fitting each

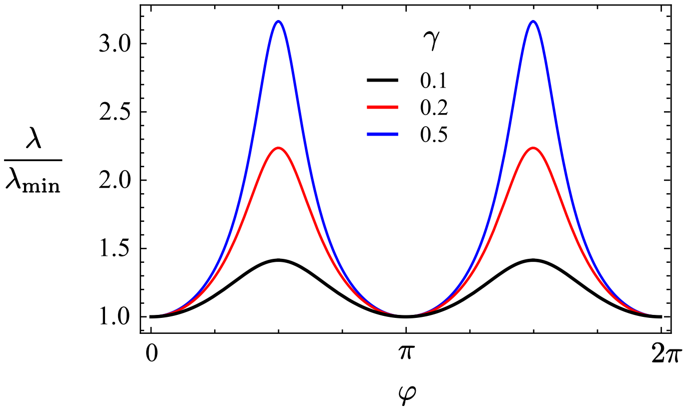


FIG. S5. Normalized cortical tension $\lambda/\lambda_{\text{min}}$, calculated as expressed by Eq. (4) in the main text, versus the turning angle $\varphi$ (see Fig. 2) for $\theta_{\text{SF}} = \pi/2$ and various $\gamma$ values. Upon increasing the anisotropy parameter $\gamma$, the cortical tension becomes progressively less uniform across the arc. Maximal tension is attained when $\varphi = \pi/2$ and the tangent vector $\boldsymbol{T}$ is parallel to the stress fibers.

ellipse separately and averaging the lengths of the axes of the ellipses. Ellipses whose $\chi^2$ is greater than 10 are discarded, which occurs in case of membrane ruffling and other out-of-equilibrium events.

In the global fit, the orientations of the ellipses are fixed to the local orientations of stress fibres. Orientations are measured from the channel with TRITC-Phalloidin (Actin) using the OrientationJ plugin for ImageJ. The average orientation per cell edge segment is calculated over all pixels between 15 and 50 pixels (2.07 µm and 6.9 µm) away from the cell edge whose coherency is greater than 0.15.

## Force analysis

Fig. S5 shows the cortical tension given by Eq. (4) in the main text as a function of the turning angle $\varphi$ and for $\theta_{\text{SF}} = \pi/2$. The isotropic limit is recovered when $\gamma = 1$ and $\lambda = \lambda_{\text{min}}$ along the entire cellular arc. For both isotropic and anisotropic cells, traction forces can be calculated by summing the cortical tension $\boldsymbol{F} = \lambda \boldsymbol{T}$ of the two arcs meeting at a specific adhesion point. In the anisotropic case, this is more conveniently done by first rotating the ellipse in such a way the minor and major axes are parallel to the $x-$ and $y-$direction respectively. Then two forces $\boldsymbol{F}_1$ and $\boldsymbol{F}_0$ are calculated by combining Eqs. (3) and (4) and defined in such a way that they are pointing clockwise and counter-clockwise around the ellipse:

$$\frac{\boldsymbol{F}_0}{\lambda_{\text{min}}} = \left(\frac{d}{2b}\sin\phi + \frac{\rho}{b}\cos\phi\right)\hat{\boldsymbol{x}} - \left(\frac{d}{2\gamma b}\cos\phi - \frac{\rho}{b}\sin\phi\right)\hat{\boldsymbol{y}}\,, \tag{S1a}$$

$$\frac{\boldsymbol{F}_1}{\lambda_{\text{min}}} = \left(\frac{d}{2b}\sin\phi - \frac{\rho}{b}\cos\phi\right)\hat{\boldsymbol{x}} - \left(\frac{d}{2\gamma b}\cos\phi + \frac{\rho}{b}\sin\phi\right)\hat{\boldsymbol{y}}\,, \tag{S1b}$$

where the distance $\rho$ is defined as:

$$\rho = \sqrt{b^2\left(\frac{1+\tan^2\phi}{1+\gamma\tan^2\phi}\right) - \frac{1}{\gamma}\left(\frac{d}{2}\right)^2}\,. \tag{S2}$$

Here $d$ is the distance between the positions of both forces on the ellipse, $b$ is the major semi-axis of the ellipse and $\phi$ is the angle that the line through both points makes with the $x-$axis (see Fig. S6). After this $\boldsymbol{F}_0$ and $\boldsymbol{F}_1$ are rotated back to the coordinate system of the image and summed to give the force, scaled by $\lambda_{\text{min}}$, acting on the cell edge on the location of a particular intersection of two ellipses.

The magnitude of the traction forces is required for the calculation of the minimal line tension $\lambda_{\text{min}}$ and the isotropic and directed stresses $\sigma$ and $\alpha$. We get this from the micropillar array. A measured force usually is the sum of two forces exerted by two different cell edge segments. Therefore, we first decompose the traction force into two forces pointing along tangents to the two cell edge segments adjacent to the position of the force. Then, per cell, we take

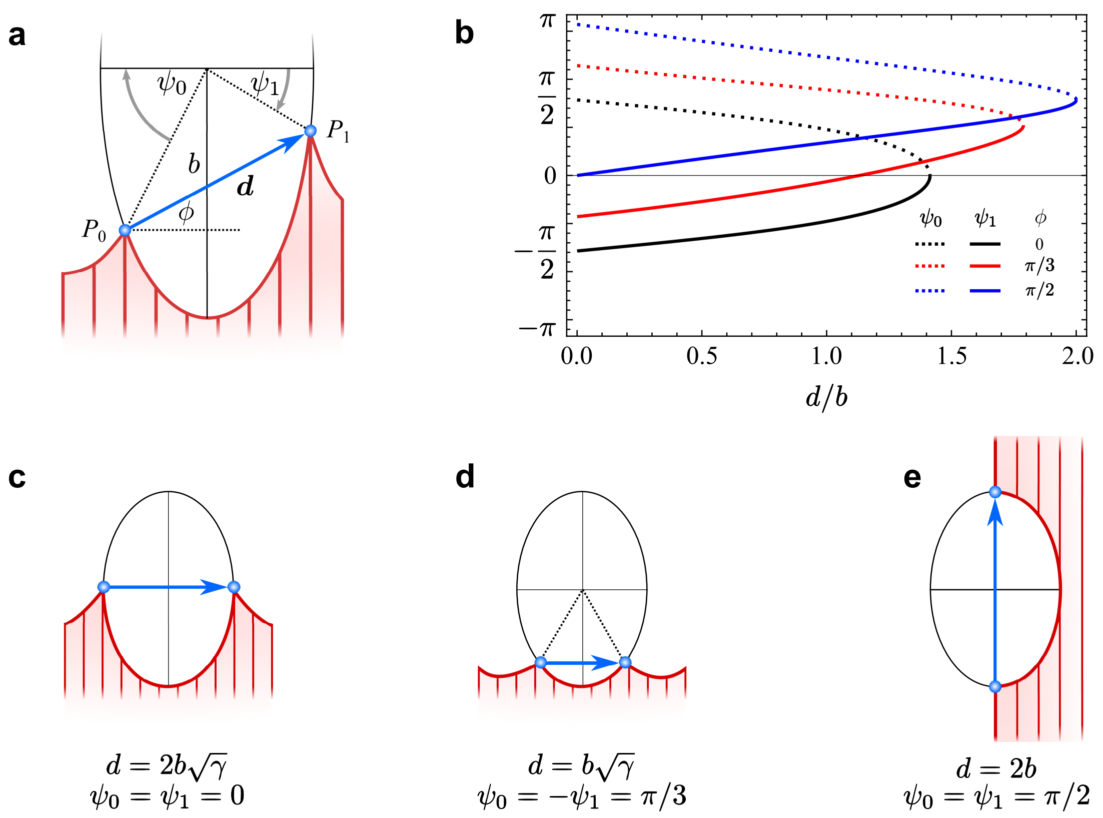


FIG. S6. Angular coordinates of the adhesion points. (a) Schematic illustration of a cellular arc and the approximating ellipse. The angular coordinates $\psi_0$ and $\psi_1$ are measured with respect to the negative and positive $x-$direction respectively. Thus, in the displayed configuration $\psi_0 > 0$ and $\psi_1 < 0$. The ellipse major semi-axis is set by the ratio between peripheral and bulk contractile stresses, i.e. $b = \lambda_{\rm min}/\sigma$. (b) Angular coordinates $\psi_0$ (dotted line) and $\psi_1$ (solid line) as a function of the rescaled distance between the adhesion points, i.e. $d/b$, for various choices of the tilt angle $\phi$ and $\sigma = \alpha$ (hence $\gamma = 1/2$). (c), (d) and (e) Examples of specific configurations for various choices of $d$ and $\phi$.

any combination of two clockwise and counter-clockwise forces and calculate:

$$\lambda_{\rm min} = \sqrt{\frac{F_{1x}^2 F_{0y}^2 - F_{0x}^2 F_{1y}^2}{F_{0y}^2 - F_{1y}^2}}\,, \qquad \sigma = \frac{|\boldsymbol{F}_0 - \boldsymbol{F}_1|}{d}\,\frac{F_{0x} + F_{1x}}{F_{0y} - F_{1y}}\,, \qquad \alpha = \sigma\left(\frac{1}{\gamma} - 1\right)\,. \tag{S3}$$

Here $\boldsymbol{F}_0$ and $\boldsymbol{F}_1$ are defined in the coordinate system where the $x-$ and $y-$axes are the minor and major axes of the ellipse. Furthermore, $F_{nx}$ and $F_{ny}$ are the components of $\boldsymbol{F}_n$ in the $x$ and $y-$directions respectively. To calculate values for these quantities, we average all the different tensions and stresses we get for all possible combinations in all cells, taking the errors on these values into account as weights while averaging.

### Angular coordinates of the adhesion points

As we explained in the main text, the ratios $b = \lambda_{\rm min}/\sigma$ between the peripheral and bulk contractility and $\gamma = \sigma/(\sigma+\alpha)$ between isotropic and directed stresses set, respectively, the major semi-axis and the aspect ratio $a/b = \sqrt{\gamma}$ of the ellipse approximating the shape of the cellular arcs, whereas the orientation of the ellipse is determined by the direction of the stress fibers. These quantities uniquely identify the ellipse, the shape and the orientation of the ellipse, but not which portion of the ellipse corresponds to a given cellular arc. In order for this to be uniquely determined, one needs to specify relative position $\boldsymbol{d} = d(\cos\phi, \sin\phi)$ of the adhesion points (Fig. S6a), where the stress fibers are assumed, without loss of generality, parallel to the $y-$axis.

Then, using Eq. (3) in the main text with $\theta_{\rm SF} = \pi/2$, one can straightforwardly calculate the coordinates of the

center of the ellipse in the reference frame centered at the first adhesion point ($P_0$ in Fig. S6a), namely:

$$x_c = \frac{d}{2}\cos\phi - \gamma\rho\sin\phi \;, \tag{S4a}$$

$$y_c = \frac{d}{2}\sin\phi + \rho\cos\phi \;. \tag{S4b}$$

From Eqs. (S4), standard algebraic manipulations allow us to express the angular coordinate $\psi$ of the adhesion points in the frame of the ellipse (Fig. S6a), namely:

$$\tan\psi_0 = \frac{d\sin\phi + 2\rho\cos\phi}{d\cos\phi - 2\gamma\rho\sin\phi} \;, \tag{S5a}$$

$$\tan\psi_1 = \frac{d\sin\phi - 2\rho\cos\phi}{d\cos\phi + 2\gamma\rho\sin\phi} \;. \tag{S5b}$$

An illustration of the possible configurations described by Eqs. (S5) is shown in Fig. S6(b)-(e). When $\rho$ becomes imaginary, the two adhesion point are as far apart as possible along the ellipse. This sets the position of the extremum of the curves displayed in Fig. S6b.

## Orientational analysis of the stress fibers

Fig. S7 shows an analysis of the stress fibers orientation (central column) and alignment (right column) for the six example cells displayed in Figs. S2, S3 and S4. The local amount of alignment, in particular, has been calculated using the ImageJ pluggin OrientationJ (http://bigwww.epfl.ch/demo/orientation), through the following procedure. Let $I(x,y)$ be the intensity of the image at the point $(x,y)$ and $I_u = \boldsymbol{u}\cdot\nabla I$, the projection on the gradient of $I$ along the arbitrary $\boldsymbol{u}$ direction. The amount of anisotropy of the image can be quantified by introducing the extrema of the squared norm of $I_u$, namely:

$$\Lambda_{\rm max} = \max_{\boldsymbol{u}} \|I_u\|^2 \;, \qquad \Lambda_{\rm min} = \min_{\boldsymbol{u}} \|I_u\|^2 \;, \tag{S6}$$

where $\|\cdots\| = \int_{\rm ROI} {\rm d}x\,{\rm d}y\,(\cdots)$ stands for the norm of a function calculated in a specific region of interest (ROI). The amount of anisotropy is then naturally quantified in terms of the coherence parameter:

$$C = \frac{\Lambda_{\rm max} - \Lambda_{\rm min}}{\Lambda_{\rm max} + \Lambda_{\rm min}} \;. \tag{S7}$$

In case of isotropic distributions, $\Lambda_{\rm max} = \Lambda_{\rm min}$ and $C = 0$. On the other hand, in case of strongly aligned stress fibers $\Lambda_{\rm max} \gg \Lambda_{\rm min}$ and $C \approx 1$. From the right column of Fig. S7, we see that the stress fibers are highly aligned in the periphery of the cell, consistently with our theoretical model.

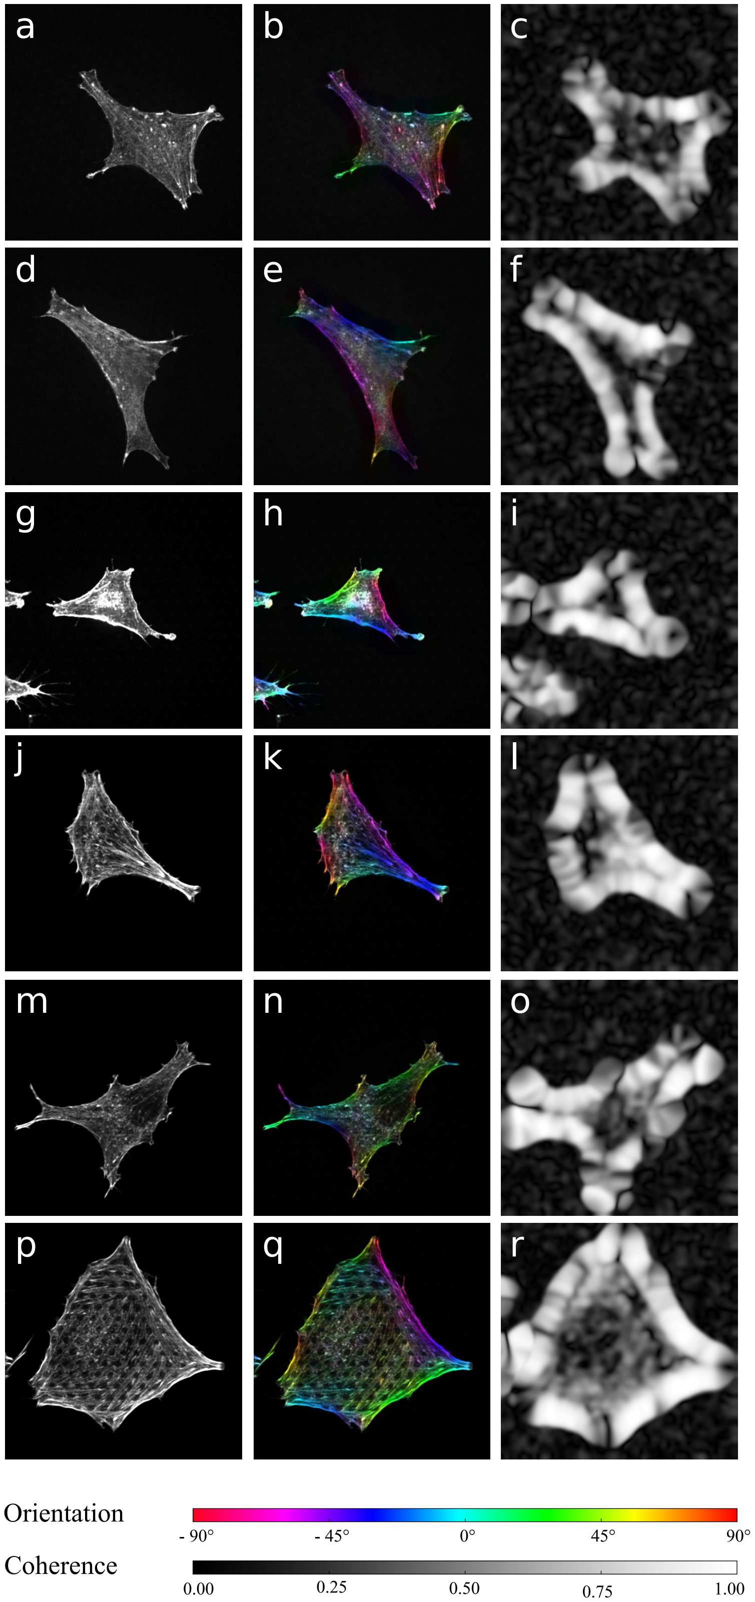


FIG. S7. Orientational analysis of the stress fibers. On the left column, optical micrographs of the six example cells displayed in Figs. S2, S3 and S4. On the center column, color survey of the stress fibers orientation. On the right column, density plot of the orientational coherence of the stress fibers, computed via OrientationJ. Along the cell periphery, stress fibers are highly aligned and the calculated coherence is close to one (see Sec. Orientational analysis of the stress fibers for details).
